# Supplementary material for: Stable hydrogenated graphene edge types: Normal and reconstructed Klein edges
Source: arXiv:1306.3384 source file (2013-09-30)
Supplement: Supplementary file 1 [file Suppl_Mat_Wagner.pdf]

# Supplementary Materials
# New stable hydrogenated graphene edge types: Klein edge and reconstructed Klein edge

Philipp Wagner,[1] Viktoria V. Ivanovskaya,[2] Manuel Melle-Franco,[3] Bernard Humbert,[1] Jean-Joseph Adjizian,[1] Patrick R. Briddon,[4] and Christopher P. Ewels[1,*]

[1]*Institut des Matériaux Jean Rouxel (IMN), Université de Nantes, CNRS UMR 6502, 44322 Nantes, France*
[2]*Unité Mixte de Physique CNRS-Thales, 91767 Palaiseau, and Université Paris-Sud, 91405 Orsay, France*
[3]*Departamento de Informática, Centro de Ciências e Tecnologias da Computação, Universidade do Minho, 4710-057 Braga, Portugal*
[4]*School of Electrical, Electronic and Computer Engineering, University of Newcastle, Newcastle upon Tyne, NE 1 7RU, United Kingdom*

All calculated edge formation energies (see Table I) are in qualitative agreement with the literature where available, and show the same stability hierarchy.

Our edge formation energies are in most cases slightly lower than calculated by Wassmann *et al.*[1]. The primary difference between the current study and those of Wassmann *et al.*[1], Koskinen *et al.*[2], Lu *et al.*[3] and Kunstmann *et al.*[4] is that our calculations use the LDA-PW92 for exchange-correlation[5]. There is a tendency for LDA to overestimate bonding and GGA to underestimate it[6], and hence the experimental formation energies are likely to lie between these two. We note that GGA parameters give slightly better atomisation energies for $sp^3$-coordinated molecules such as $CH_4$[6]. This probably explains the slightly lower edge formation energies found in our work for cases with high hydrogen densities ($sp^3$ hybridized edge configurations) such as the $a_{22}$ edge configuration, but will not change qualitatively any of the interpretation, or stability order between zigzag and Klein based edges. Recalculating the armchair $a_{22}$ configuration (including optimising both the lattice parameter and atom positions) using GGA-PBE we find an edge formation energy of -0.092 eV/Å, in very good agreement with width 10 GNRs from Lu et al. who find $E_{edge}$= -0.095 eV/Å using also GGA-PBE (if we assume a periodicity of 4.26 Å along the AGNR). It is close to -0.071 eV/Å found by Wassmann *et al.* but still slightly more stable.

It is additionally possible that the values from Wassmann *et al.* were slightly influenced due to the relatively short vacuum distances between the GNRs (8.5 Å), and the fact that the lattice parameter was fixed. When fixing the lattice parameter, we found that lattice relaxation can slightly lower the formation energy, in the range of 0.01 eV/Å. The current calculations also use $\sim$ 50 Å wide GNRs, which are wider than those in the literature. At this width interactions of the opposite edges can be excluded with certainty. For comparison, for the same small width 10 AGNR as Lu *et al.*[3], we calculate an edge formation energy using GGA-PBE of -0.101 eV/Å. This slightly more stable edge formation energy for smaller width ribbons is again in good agreement with the findings of Lu *et al.* We compared the different k-point meshes used in the studies of Wassmann *et al.*[1] and Kunstmann *et al.*[4] with the current study, and this resulted in negligible differences in energy ($<$ 0.003 eV/Å). However the choice of the basis set and pseudopotentials can also lead to small differences.

Thus differences up to 0.04 eV/Å between different calculations due to the various reasons given above, even when using the same underlying approach (e.g. GGA), are not unusual. The hierarchy in stability of the different edge configurations nonetheless remains identical.

---

* chris.ewels@cnrs-imn.fr


[1] T. Wassmann, A. P. Seitsonen, A. M. Saitta, M. Lazzeri, and F. Mauri, Phys. Rev. Lett., **101**, 096402 (2008).

[2] P. Koskinen, S. Malola, and H. Häkkinen, Phys. Rev. Lett., **101**, 115502 (2008).

[3] Y. H. Lu, R. Q. Wu, L. Shen, M. Yang, Z. D. Sha, Y. Q. Cai, P. M. He, and Y. P. Feng, Appl. Phys. Lett., **94**, 122111 (2009).

[4] J. Kunstmann, C. Ozdoğan, A. Quandt, and H. Fehske, Phys. Rev. B, **83**, 045414 (2011).

[5] J. P. Perdew and Y. Wang, Phys. Rev. B, **45**, 13244 (1992).

[6] J. P. Perdew, K. Burke, and M. Ernzerhof, Phys. Rev. Lett., **77**, 3865 (1996).

| This work | | | | | | | | Literature |
|---|---|---|---|---|---|---|---|---|
| hydrogenated graphene edge type | | $E_{edge}$ (eV/Å) | $E_{edge}$ (eV/$n_{C_{edge}}$) | $\rho_H$ ($n_H$/Å) | magnetic edge states | ($\mu_B$/Å) | ($\mu_B/n_{C_{edge}}$) | $E_{edge}$ (eV/Å) |
| $a_{11}$ | 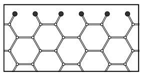 | +0.028 | +0.060 | 0.472 | No | - | - | +0.032 [a] / +0.01 [b] / +0.013 [c] |
| $a_{21}$ | 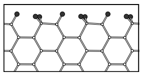 | +0.163 | +0.345 | 0.707 | Yes | 0.228 | 0.483 | +0.209 [a] |
| $a_{22}$ | 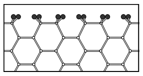 | -0.186 | -0.394 | 0.944 | No | - | - | -0.071 [a] / -0.095 [c] |
| $a_{3333}^{uudd}$ | 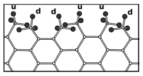 | -0.318 | -1.347 | 1.418 | No | - | - | - |
| $z_1$ | 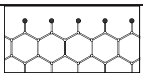 | +0.105 | +0.256 | 0.409 | Yes | 0.128 | 0.313 | +0.081 [a] / +0.06 [b] / +0.11 [d] |
| $z_2$ | 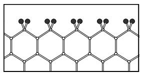 | +0.150 | +0.367 | 0.816 | Yes | 0.261 | 0.639 | +0.222 [a] |
| $z_{21}$ | 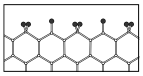 | -0.008 | -0.021 | 0.612 | No | - | - | +0.038 [a] |
| $z_{211}$ | 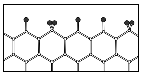 | -0.016 | -0.040 | 0.545 | No | - | - | +0.012 [a] / +0.03 [d] |
| $rk_{11}$ | 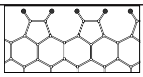 | +0.302 | +0.737 | 0.409 | No | - | - | - |
| $rk_{22}$ | 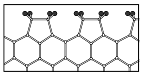 | -0.030 | -0.072 | 0.820 | Yes | 0.120 | 0.292 | - |
| $rk_{21}$ | 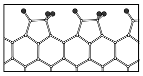 | +0.134 | +0.328 | 0.614 | No | - | - | - |
| $rk_{22} + k_2$ | 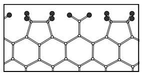 | +0.034 | +0.083 | 0.818 | No | - | - | - |
| $rk_{22} + z_2$ | 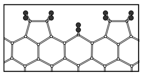 | -0.107 | -0.261 | 0.818 | No | - | - | - |
| $k_1$ | 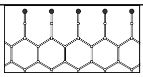 | +1.276 | +3.116 | 0.409 | No | - | - | - |
| $k_2$ | 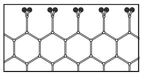 | +0.476 | +1.160 | 0.820 | No | - | - | - |
| $k_{32}$ | 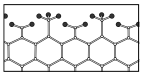 | +0.052 | +0.128 | 1.022 | No | - | - | - |
| $k_{33}^{ud}$ | 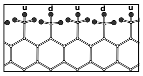 | -0.150 | -0.367 | 1.227 | Yes | 0.108 | 0.263 | - |
| $k_{332}^{ud}$ | 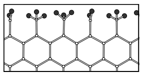 | +0.490 | +1.203 | 1.089 | Yes | 0.098 | 0.241 | - |
| $k_{33}^{ud} + z_2$ | 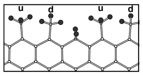 | -0.191 | -0.467 | 1.086 | No | - | - | - |

*a*: Wassmann *et al.*[1], *b*: Koskinen *et al.*[2], *c*: Lu *et al.*[3] (*a-c* all GGA-PBE), *d*: Kunstmann *et al.*[4] (GGA-PW91)

TABLE I. Edge formation energies, edge hydrogen density $\rho_H$ and magnetic moment given for different hydrogen terminated armchair, zigzag, reconstructed Klein and Klein edges. For all hydrogenated edge configurations the strain $\epsilon$ parallel to the edge, compared to pristine graphene, has been found to be small ($\epsilon \leq \pm 0.3\%$) for all optimised relaxed structures. Thus changes of the ribbon properties due to strain, induced by hydrogen termination, can be excluded. $n_{C_{edge}}$: number of edge carbon atoms.
